# Supplementary material for: Do End-to-end Stereo Algorithms Under-utilize Information?
Source: arXiv:2010.07350 source file (2020-10-14)
Supplement: Supplementary file 1 [file supp-runtime.tex]

\begin{table*}[t]
\small
\centering
\scalebox{0.96}{
    %\begin{tabularx}{1.0\linewidth}{p{0.75cm} | XX XX XX XX}
    %\begin{tabularx}{1.0\linewidth}{@{} p{0.75cm} | YYY| YYY |YYY | YYY @{}}
    \begin{tabularx}{1.0\linewidth}{@{} ?{1pt} p{0.75cm} ?{1pt} YY ?{1pt} YY  ?{1pt}YY ?{1pt} YY ?{1pt} @{}}
    %\hline
    \Xhline{2\arrayrulewidth}
	\multirow{3}{0.8pt}{{\bf Filters}} & \multicolumn{2}{c ?{1pt} }{ \bf DispNetC} & \multicolumn{2}{c ?{1pt}  }{ \bf PSMNet}  & \multicolumn{2}{c ?{1pt}  }{ \bf GANet} & \multicolumn{2}{c ?{1pt}}{ \bf GCNet} \\
	\cline{2-9} % draw a horizontal line spanning only some of the table cells
	%&\multicolumn{8}{c}{Bad-3.0 Error Rates (\%)}  \\
	 &{Mem.(MiB)}  &{Time (ms)}  &{Mem.(MiB)}  &{Time (ms)} &{Mem.(MiB)}  &{Time (ms)} &{Mem.(MiB)}  &{Time (ms)} \\
	%\hline \hline
	\Xhline{2\arrayrulewidth}
	\hline
	W/O & \textbf{1394} & \textbf{18.35}  & \textbf{5151} &\textbf{ 315.57}  & \textbf{7178 }& \textbf{1894.70}  & \textbf{4280} & \textbf{146.83}  \\
	\hline
	%\Xhline{2\arrayrulewidth}
	\cellcolor{myskyblue} SABF  & 1888 & 24.32  & 5386 & 563.42  & 7920 & 2488.72  & 4424 & 379.37   \\
	\cellcolor{myskyblue} DFN & 1422 & 28.33  & 5246 & 432.32  & 7466 & 2041.53  & 4298 & 255.20   \\
	\cellcolor{myskyblue}PAC & 1535 & 25.34  & 5168 & 514.91  & 8274 & 2383.44  & 4400 & 334.73   \\
	%\cellcolor{myskyblue}SGA & \cellcolor{mygray}\textbf{0.57} & \cellcolor{mygray}\textbf{9.37} & \cellcolor{mygray}\textbf{3.21} & \cellcolor{mygray}0.40 & \cellcolor{mygray}6.08 & \cellcolor{mygray}2.14  &- &- &-  & \cellcolor{mygray}\textbf{0.55} & \cellcolor{mygray}\textbf{9.24} & \cellcolor{mygray}\textbf{2.98}  \\
	\cellcolor{myskyblue} SGA & 7066 & 489.60  & 11070 & 823.00  & - & -  & 9916 & 655.18 \\
	%\hline
	\Xhline{2\arrayrulewidth}
	
	\end{tabularx}}
\vspace{-4pt}
\caption{Runtime (ms) and GPU memory consumption (MiB). Results are shown in the entries of filters (rows in skyblue) and backbones (columns) w.r.t. the baselines (rows W/O). The smallest values are in bold. GANet already contains SGA, resulting in blank entries ``-''.
}
\label{tab:kt15-all-runtime}
\end{table*}
